# Supplementary material for: FLEX: Extrinsic Parameters-free Multi-view 3D Human Motion Reconstruction
Source: arXiv:2105.01937 source file (2022-10-21)
Supplement: Supplementary file 1 [file sup_network_structure.tex]

\input{LaTeX/figures/layer_detail}

\sout{We now describe the full architecture of each component, $F_Q$, $E_Q$, $F_S$, $E_S$ and $D$. The parameters of each layer are detailed in \cref{tab:layer_detail}.

Both fusion components $F_Q$ and $F_S$ start with a channel-expansion layer, followed by a view-fusion block, and completed by a transformer encoder {\color{orange}multi-head attention layer} that attends views.}
%In both $F_S$ and $F_Q$ there are three main parts: channel-expansion, information-fusion and view-wise attention.
\sout{
Channel-expansion is done using convolutional layers with a kernel of size 1.
%In the expansion part we use convolutional blocks, where the convolutions have kernel size 1 and stride 1. 
In the view-fusion part, for $F_Q$, we apply three parallel 2D convolutional kernels with different kernel sizes, followed by adaptive average pooling. For $F_S$, we use sequential convolutional layers.

Our view-transformer block is based on the  LiftFormer transformer encoder and contains two transformer encoder layers with two heads each. Each transformer encoder is composed of two self attention layers with layer norm. 
The result of applying the view-transformer is that the view dimension collapses (visualized in \cref{fig:architecture_detail}).}
{\color{orange}\sout{
Our view-attention block is composed of 64 attention heads. The result of applying the view-attention is that the view dimension collapses (visualized in \cref{fig:architecture_detail}).}}

\sout{The encoder block $E_Q$ consists of three parallel 1D convolutional layers of different kernel sizes, followed by a final additional 1D convolution. The encoder $E_S$ starts with an adaptive max pooling to collapse the time dimension and then runs a final 1D convolution.

%and then collapse all the temporal information into a single vector with adaptive max pooling. Then for both branches we apply a view-wise transformer encoder composed of 2 layers that each contains a 2-heads attention block.
 
Our discriminator $D$ is a linear component that contains two convolution layers and one fully connected layer, based on Kanazawa~\etal~\shortcite{Kanazawa:2018}). Its output value is between 0 and 1.  
%for each rotating joint, that is, a joint that is not an end effector.as there are joints that are end-effectors which means they don't have any rotation in the human kinematic chain, so their rotation angle is not predicted by our network. 
 
After each convolution block, we apply batch normalization, a leaky rectified linear unit and dropout. 
%The kernel width and the stride are denoted by $k$ and $s$, respectively, and the number of input and output channels is given in the rightmost column.}{}
}
